# Supplementary material for: Knodle: Modular Weakly Supervised Learning with PyTorch
Source: arXiv:2104.11557 source file (2021-07-04)
Supplement: Supplementary file 1 [file 9_appendix.tex]

%\newpage
\appendix
%\section{Appendix}

\section{Code example}
\label{sec:code}
The following code snippet shows a minimal example of the usage of the Knodle framework.
It demonstrates an end-to-end process, starting from data loading, training, evaluation and model storage.
Of course, the \texttt{Config} class and its inheriting classes take many more parameters, such as batch size or various options to handle cases where no rule matches discussed in~\ref{subsec:neg_samples}.

\small

\lstinputlisting[language=Python]{pythoncode.py}
